# Supplementary material for: Sim-to-Real Learning of All Common Bipedal Gaits via Periodic Reward Composition
Source: arXiv:2011.01387 source file (2021-03-11)
Supplement: Supplementary file 1 [file appendix.tex]

Helloooo

$$f(x) = x$$
